# Supplementary material for: Quantum Coherence is Preserved in Extremely Dispersive Plasmonic Media
Source: arXiv:1810.00114 source file (2019-05-01)
Supplement: Supplementary file 1 [file PhysRevApplied_Supplement.pdf]

# Supplemental Materials for:

# Quantum Coherence is Preserved in Extremely Dispersive Plasmonic Media

Yury S. Tokpanov[1], James S. Fakonas[1], Benjamin Vest[1], and Harry A. Atwater[1*]

## Affiliations

[1]Thomas J. Watson Laboratories of Applied Physics, California Institute of Technology, Pasadena, California 91125.

## Elliptical hole array in the linear regime

In this part, we investigate the preservation of quantum entanglement when sending photons through a hole array when excited plasmons are “photon-like”, i.e. when choosing an operating point on the dispersion relation close to the light line. To do so, we designed, fabricated and characterized a hole array sample dedicated to the excitation of plasmons at the interface between gold and glass. As a warm-up experiment, we study the influence of the hole geometry on the preservation of quantum entanglement. This experiment gives us a reference point to initiate a comparison with plasmon excitation in the highly-dispersive regime, as performed in the main paper.

To study geometrical effects, we used a plasmonic array of elliptical holes milled through a 200 nm thick layer of gold deposited on a glass substrate, by using a focused ion beam with purposely-introduced astigmatism. The dispersion relation of the gold-glass interface was computed from an analytical modal dispersion model (see Fig S1). A first choice for the hole dimensions and the array periodicity was made after numerical simulations of the structure designed to enhance extraordinary transmission at 812 nm – the wavelength of our down-converted photons. The sample we used had a size 1 mm x 1 mm and was fabricated in a clean room environment. Its transmission was enough to detect satisfying level of signal. The hole shape in these arrays is close to elliptical, with axes equal to 240nm and 190nm (see Fig. S2(A)). The difference between those two dimensions makes the optical transmission of this sample polarization-dependent (Fig. S2(B)). This sample has linear SPP dispersion (Fig. S1), so that we could focus on hole geometry effects only in this experiment.

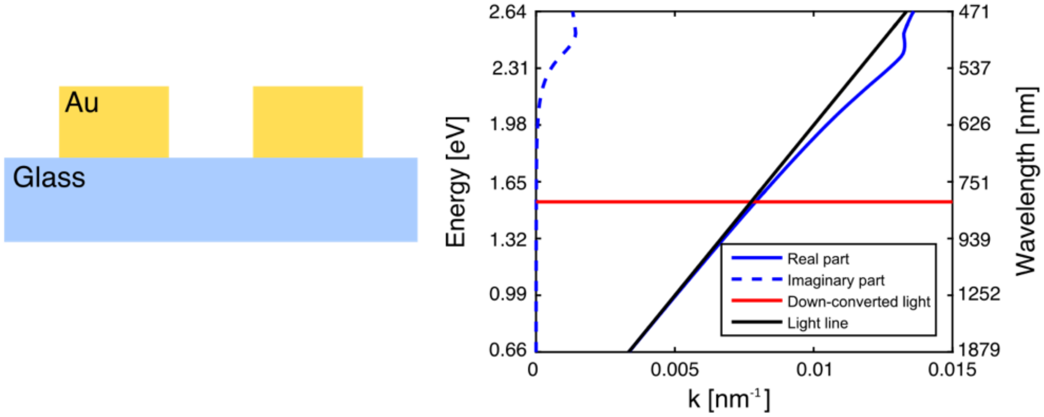


**Figure S1. Design of plasmonic elliptical hole array.** Cross-sectional schematic and dispersion relation of elliptical hole arrays for SPPs supported at the gold/glass interface. At the wavelength of the down-converted photons (812 nm, as shown by the red solid line), the dispersion is ‘photon-like’, i.e., linear and very close to the light line.

First, we performed a measurement using polarization entangled light (Fig. S2(C)) (rotating a sample in such a way that hole array eigenmodes directions were along the vertical and horizontal polarizations). The transmission of the first channel (considered as an influence of the environment on the system) being now polarization dependent, we expect the two terms of the state in Eq. (3) of the main paper to be differently affected by the insertion of the plasmonic array, and thus a reduction of the visibility. In both we found the visibility of curves, corresponding to the mixture of eigenmodes ($\beta = 45^\circ$ and $\beta = 135^\circ$ on Fig. S4(C)) of hole array, to be $V = 86\% \pm 5\%$.

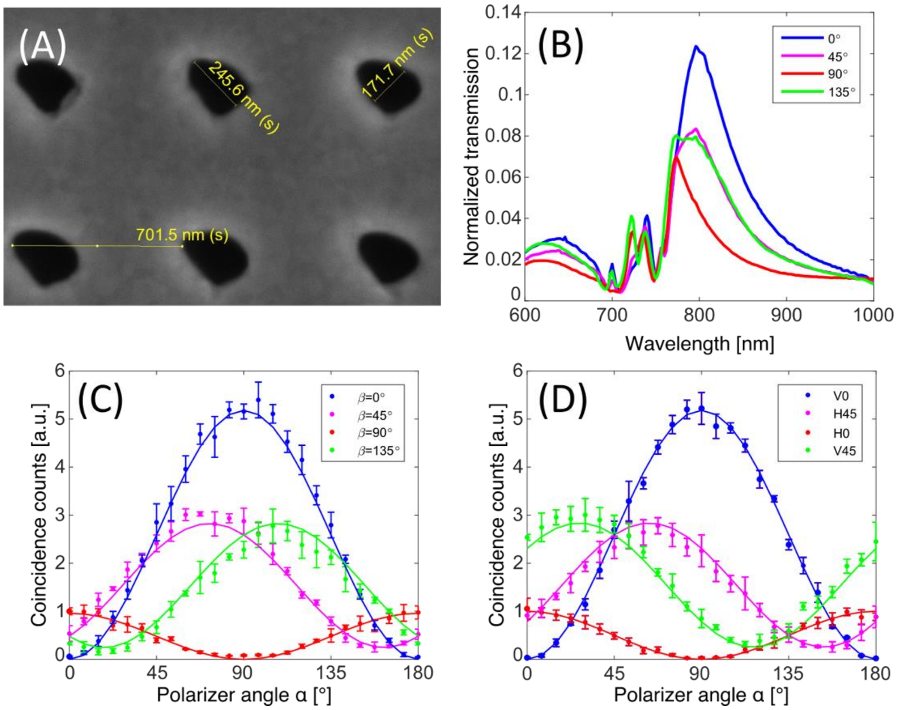


**Figure S2. Study of entanglement preservation with the elliptical hole array.** Elliptical hole array used to study the influence of hole geometry on the preservation of photon entanglement: **(A)** SEM image, where the orientation of the minor and major axis can be seen oriented at +/- 45°; **(B)** Transmission factor of the device for different polarizations of incident light. The holes have no rotation symmetry anymore, so that the transmission maximum varies between 12.5 % for horizontally polarized light and 7% for vertically polarized light. **(C)&(D)** Normalized number of coincidence counts as a function of polarizer angles in the presence of an elliptical plasmonic hole array (solid line represents fit to the full model) in two configurations : **(C)** With entangled photons and for different fixed directions of the polarizer beta; **(D)** With classical light and similar choice for beta. The plots with β= 45° and β=135° show a similar decrease in visibility in both configurations, indicating that this results from a purely classical effect.

However, we need to determine to what extent this reduction is caused by the quantum mechanical decoherence (through a decrease of the overlap factor $V = |\langle E_V | E_H \rangle| \cos(\Delta\varphi_E + \Delta\varphi)$, provided $\Delta\varphi_c = 0°$) or by the modification of the complex transmission ratio v/h, which is a purely classical effect. In order to do so, we performed a control experiment using classical light, in which we generated just unentangled polarized photon pairs, either in the pure $|H, H\rangle$ state, or in the pure $|V, V\rangle$ state.(Fig. S2(D)). To record Fig. S2(D) we first fixed the hole array at exactly the same rotation as used in Fig. S2(C) and transmitted horizontal and then vertical polarizations (H0, V0 curves on Fig. S2(D) correspond to $\beta$=0˚ and $\beta$=90˚ on Fig. S2(C)). The amplitude ratio between the two sine curves is an indication of the ratio of the transmission amplitudes of horizontal and vertical polarizations through the hole array |h/v|. Then we rotated the hole array by 45˚ and repeated the measurement (H45, V45 curves on Fig. S2(D)) correspond to $\beta$=45˚ and $\beta$=135˚ on Fig. 2(C)). In this configuration, the hole array behaves as a birefringent plate whose axis are at 45° with respect to the polarization of the incident photon. The dephasing and the transmission ratio between the two eigenpolarizations can be related to the azimuth and the ellipticity of the output polarization of the photon. From the measurement with classical light and by fitting the different plots of Fig. S2(D), we determined $\frac{|h|}{|v|} = 5.2 \pm 0.3$ and $\Delta\varphi = 48° \pm 4°$. Substituting these values to Eq.(3) and fitting (3) to curves on Fig. S2(C) gives $|\langle E_V | E_H \rangle| = 1.0 \pm 0.1$ and, $\Delta\varphi_E = 1° \pm 4°$so that within experimental error we did not detect quantum mechanical decoherence.

Breaking the symmetry of the hole shape introduces distinguishability between the eigen polarizations of the problem and degrade the visibility of interferences. However, the reported decrease in visibility is strictly analogous to the classical situation of an unbalanced interferometer, where two waves of non-equal amplitudes interfere, leading to non-optimal fringe contrast. The reduction of visibility is, in this case, a purely classical effect.

## Non-linear dispersion regime of the fabricated structures

We present here further analysis that we performed to confirm that the fabricated hole arrays display characteristics that match the numerical simulations performed for the design of the structure.

The direct comparison of the transmission spectrum at normal incidence of a single structure with the simulated data is made difficult by the overall extreme sensitivity of surface plasmons to geometric defects and roughness of the different layers (intrinsically related to the limits of the fabrication process), that were not included in the numerical model of the structure (performed using only perfectly flat layers). These effects result in a broadening of the transmission peaks in the experimental data, that complicates the identification of the different resonances.

In order to overcome this difficulty, we fabricated a set of hole arrays with different periodicity ranging from 600 nm to 1000 nm, following the same fabrication procedures (resulting in the same film thicknesses and hole diameters). The period of the structures defines the wavevectors of plasmons that can couple to the structures. Overall, and thanks to the reproducibility of the fabrication processes, the acquisition of transmission spectra at normal incidence for these different structures can be seen as an indirect measurement of the dispersion relation of the structure. The next step of our approach consists in comparing these experimental transmission spectra of the different hole array structures with the analytical dispersion relation displayed on Fig. 3 of the main paper, and to check if the evolution of their respective characteristics (in practice, evolution and spectral shift of the resonance maxima) are compatible with each other.

Figure S3 displays an interpolation of a set of transmission spectra obtained experimentally for the nine different structures (color map). The operating point of our main experiment, with a structure of periodicity 850 nm and a plasmon energy around 1.52 eV, is marked with a black cross. The map displays different branches, i.e. different sets of plasmon energies and wavevectors that fulfill a resonant condition, all excited in parallel when performing our experiment, and corresponding to different folded portions of the dispersion relation of the structure.

In first approximation, the resonance condition fulfilled by plasmons propagating in the structure can be expressed as:

$$\sqrt{2}p = d + 2\pi n/k \qquad (1)$$

where p is the period of the structure, d is the hole diameter, k is the plasmon momentum and n is an integer. The factor $\sqrt{2}$ takes into account the fact, that in our experiment hole array plasmon eigenmodes propagate along diagonal directions. SEM images and measurements show that two values must be considered for the holes diameter. The diameter of the holes in the upper aSi layer is d=430 nm and is associated to plasmons propagating along the upper aSi-gold interface. The FIB milling process produced smaller holes in the lower aSi layer, with a diameter d=300nm, this value being this time associated to plasmons propagating along the lower gold-aSi interface. Using the analytical dispersion relation of Fig. 3 to relate the plasmon momentum k and the plasmon energy, we plot the relation (1) on Fig S3 for different values of n and different values of the hole diameter. We see that we have great agreement between our experimental data and the model of (1) for different branches, and in particular for the plasmon resonance that we exploit in our experiments (branch labeled "P0" of the colormap including the black cross) when considering n=6 and d=300nm for the bottom plasmon (blue solid line) and n=5, d=430nm for the top plasmon (red solid line). We emphasize that, while we can in theory expect two different resonances for the two plasmons propagating in the structure, or in other words two sets of branches, in practice, both are significantly broadened and merge into each other. It is not possible to resolve them separately and "P0" displays only one local transmission maximum although it contains the contribution of both top-propagating plasmons and bottom-propagating plasmons.

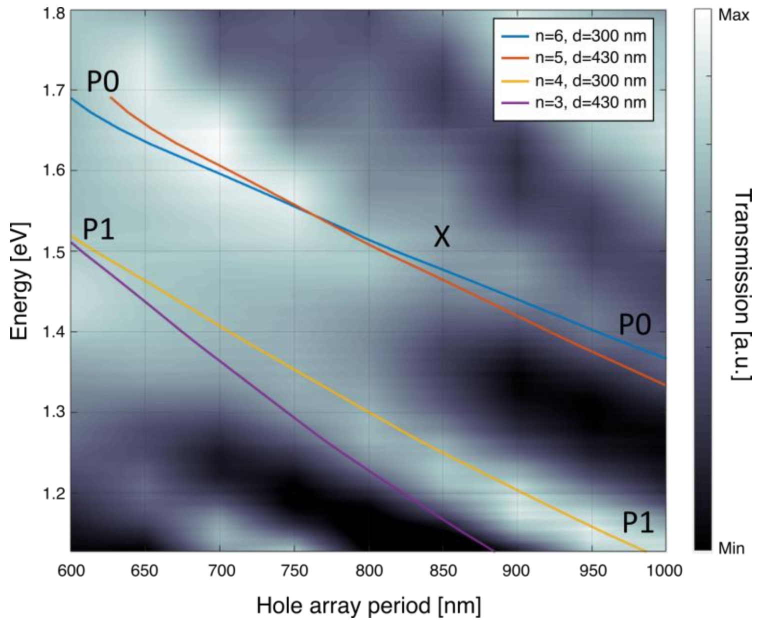


**Figure S3. Investigation of the evolution of the transmission resonances for various structures.** The transmission spectra at normal incidence of nine different hole array structures, with periods ranging from 600 nm to 1000 nm have been experimentally measured. The transmission amplitude is displayed as a color map, and as a function of both the energy (vertical axis) and of the periodicity of the hole array (horizontal axis). Experimental data have been interpolated between the nine sets of data points. The different white branches displayed on the colormap correspond to transmission resonances. The branch corresponding to the plasmon resonance exploited in the main experiment is labeled as P0 and the operating point of the experiment (structure periodicity of 850 nm, plasmon resonance at 812 nm) is marked with a black X. Another branch of plasmon resonance at lower energies is identified as P1. These branches were fitted using relation (1) for different sets of parameters (solid color lines). For both P0 and P1 agreement between experimental data and model is good and allows us to determine the plasmon wavevectors at resonance.

The parameters n and d allow us to identify the proper fraction of the dispersion relation that has to be compared with our transmission measurements. Using relation (1) and the parameters n=6 and d=300nm, we now plot on Fig. S4 our experimental transmission measurements as a function of plasmon energy and $k = \frac{2\pi n}{\sqrt{2}p - d}$ , the wavevector corresponding to the excitation of the plasmons belonging to P0, and we superimpose on the same plot the dispersion relation of Fig 3. This choice of plot highlights the agreement between or experimental data and the initial numerical design of the structure.

We finally check the robustness of our model by unfolding further the data of the transmission spectra and comparing them with the analytical dispersion relation on a larger wavevector scale. We consider, for each of the nine transmission spectra obtained with the nine experimentally characterized structures (vertical cross sections of figure S3), the wavelengths of the two local transmission maxima corresponding to both branches P0 and P1. As previously discussed, each one of these transmission peaks merges the contribution of the two plasmons propagating in the structure, either along the top or along the bottom gold-aSi interface. On Fig S5, we compare our experimental measurement of the different transmission maxima for the different structures with the analytical dispersion relation (black solid line). Each transmission maximum that was experimentally measured in the different spectra is represented as two data points placed at the same plasmon energy, but at the two different wavevectors corresponding to the top plasmon and the bottom plasmon. The values of the two plasmon wavevectors were derived using the relation (1) with the two sets of parameters (n,d) associated to P0 or P1. We can see that this unfolding procedure shows great agreement between our experimental spectra and the dispersion relation for the two major resonance branches that could be observed.

We can conclude that, taking into account geometrical defects and possible small discrepancy in optical constants between experimental and literature values used in simulations, the experimental dispersion relation is compatible with our analytical model, and that the chosen operating point at 812 nm for the structure with a periodicity of 850 nm corresponds with a surface plasmon following the intended resonance far from the light line, in the highly-dispersive regime.

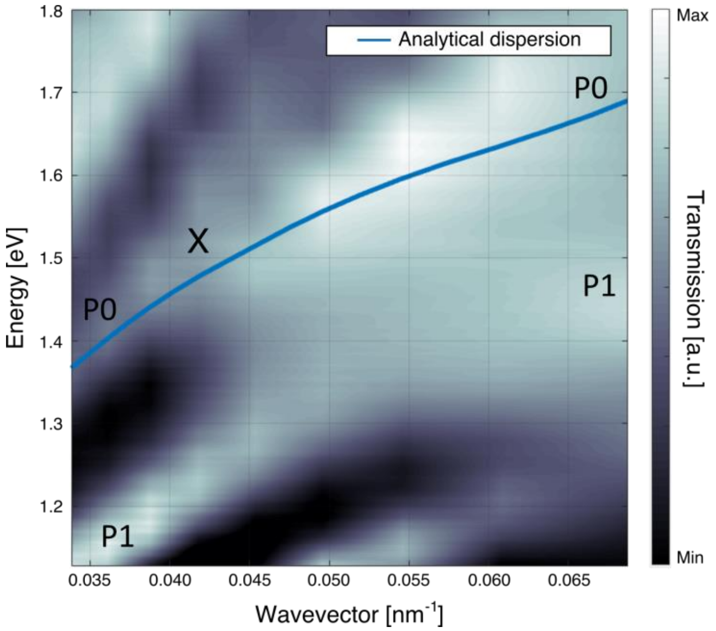


**Figure S4. Comparison of the analytical dispersion relation with the transmission measurements.** The colormap of Fig S3 is represented this time as a function of the wavevector, using the conversion between periodicity of the structures and resonant wavevectors given by relation (1) with n=6 and d=300nm. The two branches P0 and P1 are identified on the plot, as same as the operating point of the main experiment marked with a black X. P0 is well fitted by a segment of the dispersion relation that corresponds to a non-linear highly-dispersive regime for the plasmons (blue solid line), and the position of the operating point is in agreement with the initial design of the experiment.

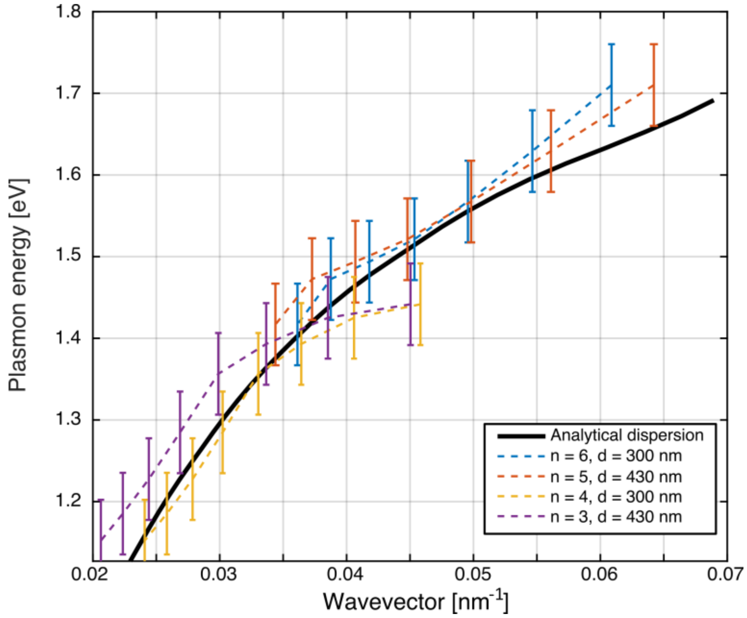


**Figure S5. Unfolding the transmission spectra to measure indirectly the dispersion relation.** We compare the analytical dispersion relation (black solid line) of the structure with the position of the local transmission maxima measured experimentally with structures of various periodicities (vertical cross sections of fig S1). For each measured transmission maximum, two values of associated wavevector are derived, by using (1) with two sets of parameters. If the transmission maximum belongs to the branch P0, the two wavevectors values are calculated using n=6, d=300nm (dashed blue line) or n=5, d=430 nm (dashed red line). If the transmission maximum belongs to the branch P1, the two wavevectors values are calculated using n=4, d=300nm (dashed yellow line) or n=3, d=430 nm (dashed purple line). This shows that experimental transmission spectra are in great agreement with the expected dispersion relation.
